# Supplementary material for: Plasmon-Polaritons in Nanoparticle Supercrystals: Microscopic Quantum Theory Beyond the Dipole Approximation
Source: arXiv:2104.08089 ancillary file (2021-04-16)
Supplement: Supplementary file 1 [file SupplMaterial.pdf]

# Supplementary Information
## Plasmon-Polaritons in Nanoparticle Supercrystals: Microscopic Quantum Theory Beyond the Dipole Approximation

Eduardo B. Barros, Bruno G. Vieira, Niclas S. Mueller and Stephanie Reich

April 13, 2021

# Contents

**1 Quadrupole Canonical Transformation** **4**

**2 Light-Matter Interaction for Dipole and Quadrupole Excitations** **6**

2.1 Taylor's Series Expansion . . . . . . . . . . . . . . . . . . . . . . . . . . . . . 7

2.2 Spherical Harmonics Expansion . . . . . . . . . . . . . . . . . . . . . . . . . . 8

**3 Nanoparticle Supercrystals** **10**

3.1 Plasmon-Plasmon Interaction . . . . . . . . . . . . . . . . . . . . . . . . . . . 10

3.2 Plasmon-Photon Interactions . . . . . . . . . . . . . . . . . . . . . . . . . . . 15

**4 Bogoliubov Transformation** **20**

**5 Quasistatic Properties** **22**

**6 Umklapp Effects** **23**

Table 1: List of Variables

| Symbol | Description | Equation/Value |
|---|---|---|
| $\rho$ | Nanoparticle radius | |
| $N$ | Number of free electrons in the nanoparticle | |
| Q | Total nanoparticle charge | $-Ne$ |
| $M$ | Total nanoparticle elecron mass | $Nm$ |
| $V$ | Nanoparticle volume | $\frac{4\pi\rho^3}{3}$ |
| $\epsilon_d$ | Metal high frequency dielectric constant | |
| $\omega_p$ | Metal plasma frequency | $\sqrt{\frac{Ne^2}{Vm\epsilon_0}}$ |
| $\epsilon_m$ | Dielectric constant of the surrounding medium | |
| $\vec{h}$ | Dipole canonical position | $\frac{1}{N}\sum_n \vec{r}_n$ |
| $\vec{\pi}$ | Dipole canonical momentum | $\sum_n \vec{p}_n$ |
| $\vec{r}'$ | Relative position | $\vec{r}' = \vec{r} - \vec{h}$ |
| $\vec{p}'$ | Relative momentum | $\vec{p} - \vec{\pi}$ |
| $H_\gamma$ | Quadrupole canonical position | $\frac{1}{N\bar{\rho}}\sum_n \chi_\gamma : \vec{r}'_n \vec{r}'_n$ |
| $\Pi_\gamma$ | Quadrupole canonical momentum | $\frac{1}{\bar{\rho}}\sum_n \chi_\gamma : \vec{p}'_n \vec{r}'_n$ |
| $\bar{\rho}$ | Expectation value of $\langle r^2 \rangle$ | $\sqrt{\frac{2}{5}}\rho$ |
| $\chi$ | Symmetric unit matrices | Eq. (S.1.8) |
| $\omega_D$ | Bare dipole oscillation frequency | $\frac{\omega_p}{\sqrt{\epsilon_d + 2\epsilon_m}}$ |
| $\omega_Q$ | Bare quadrupole oscillation frequency | $\frac{\omega_p}{\sqrt{\epsilon_d + (3/2)\epsilon_m}}$ |
| $\mathrm{Q}_D$ | Dipole effective screened charge | $\mathrm{Q}\frac{3\epsilon_m}{\epsilon_d + 2\epsilon_m}$ |
| $\mathrm{Q}_Q$ | Quadrupole effective screened charge | $\mathrm{Q}\frac{(5/2)\epsilon_m}{\epsilon_d + (3/2)\epsilon_m}$ |
| $\vec{R}$ | Real lattice vector | |
| $V_{uc}$ | Unit cell volume | |
| $\bar{R}$ | Length scale | $V_{uc}^{1/3}$ |
| $\vec{G}$ | Reciprocal lattice vector | |
| $F$ | Fill factor | $V/V_{uc}$ |
| $F_0$ | Maximum Fill factor for a given lattice | 0.74 for FCC |
| $f$ | Fill fraction | $F/F_0$ |

Table 2: List of Variables (cont.)

| Symbol | Description | Equation/Value |
|---|---|---|
| $j$ | Index for different particles in the unit-cell | |
| $\nu$ | Bare plasmon indices | 1-8 |
| $\bar{\nu}$ | Dipole or quadrupole nature of the plasmon | $D$ for $\nu = 1-3$<br>$Q$ for $\nu = 4-8$ |
| $\Lambda_D$ | Dipole coupling constant | $\frac{(\mathrm{Q}_D)^2}{8\pi\epsilon_0\epsilon_m M\omega_D V_{uc}}$ |
| $\Lambda_Q$ | Quadrupole coupling constant | $\frac{(\mathrm{Q}_Q\bar{\rho})^2}{8\pi\epsilon_0\epsilon_m M\omega_Q V_{uc}^{5/3}}$ |
| $S_{\nu\nu'}^{\bar{\nu}\bar{\nu}'}(\vec{q})$ | Plasmon-plasmon structure function | Eqs. (S.3.16),<br>(S.3.23) and (S.3.29) |
| $\mathrm{f}_D(q\rho)$ | Dipole form factor | $\frac{3}{(q\rho)^3}\left[\sin(q\rho) - q\rho\cos(q\rho)\right]$ |
| $\mathrm{f}_Q(q\rho)$ | Quadrupole form factor | $\frac{9}{(q\rho)^3}\left[\mathrm{Si}(q\rho) - \sin(q\rho)\right]$ |
| $\mathrm{Si}(x)$ | Sine integral function | $\int_0^x dz \frac{\sin(z)}{z}$ |
| $\xi_0^{\bar{\nu}}(\vec{q})$ | Plasmon-photon coupling constant | $\sqrt{\frac{2\pi\Lambda_{\bar{\nu}}}{\omega_{pt}(\vec{q})}}$ |
| $\xi_{\lambda\vec{G}}^{\nu,j}(\vec{q})$ | Plasmon-photon coupling functions | Eqs. (S.3.59), (S.3.60) |
| $\Xi_{\vec{G}\vec{G}'}^{\lambda\lambda'}(\vec{q})$ | Second-order plasmon-photon coupling | $\sum_{\nu,j}\omega_{j,\bar{\nu}}\xi_{\lambda'\vec{G}'}^{\nu,j*}(\vec{q})\xi_{\lambda,\vec{G}}^{\nu,j}(\vec{q})$ |
| $P_{\nu,\lambda}^{D}(\vec{q})$ | Dipole polarization function | $\hat{e}_\nu \cdot \hat{e}_\lambda$ |
| $P_{\nu,\lambda}^{Q}(\vec{q})$ | Quadrupole polarization function | $\frac{1}{2}[\chi_\nu : \hat{e}_q\hat{e}_\lambda + \hat{e}_\lambda\hat{e}_q]$ |

In this supplementary file we provide a detailed derivation and discussion of our microscopic theory. We also extend our theory to supercrystals with more than one particle in the unit cell. In the last section we discuss the importance of Umklapp effects in the calculation of the plasmon-polariton band structure.

# 1 Quadrupole Canonical Transformation

The problem of obtaining a canonical transformation for the quadrupole modes dates back to the description of the nucleon interactions.[1] Even though it remains an open issue, we aim to propose a concise theory.

We assume a spherical particle with radius $\rho$. The electrons in this particle are described by their dynamical position $\vec{r}_n$ with associated conjugate momentum $\vec{p}_n$. We now define new coordinates

$$h_\sigma = \frac{1}{N}\sum_n r_{n,\sigma},\ H_\gamma = \frac{1}{N\bar{C}}\sum_{n,\alpha,\beta} r'_{n,\alpha} r'_{n,\beta}\chi^\gamma_{\alpha\beta}, \tag{S.1.1}$$

and momenta

$$\pi_\sigma = \sum_n p_{n,\sigma},\ \Pi_\gamma = \frac{1}{\bar{C}}\sum_{n,\alpha,\beta} p'_{n,\alpha} r'_{n,\beta}\chi^\gamma_{\alpha\beta}, \tag{S.1.2}$$

where $N$ is the total number of charges in the particle, $r'_{n\alpha} = r_{n\alpha} - h_\alpha$ and $p'_{n\alpha} = p_{n\alpha} - \pi_\alpha$. The constant $\bar{C}$ and the matrices $\chi_\gamma$ in the dyadic $\chi^\gamma_{\alpha\beta} = \hat{e}_\alpha \cdot \chi_\gamma \cdot \hat{e}_\beta$ will be determined by imposing that these dynamical variables represent a set of canonical coordinates.

The following commutation relations need to be fulfilled

$$\begin{aligned}
\text{(i)}[h_\sigma, h_{\sigma'}] &= 0\\
\text{(ii)}[\pi_\sigma, \pi_{\sigma'}] &= 0\\
\text{(iii)}[h_\sigma, \pi_{\sigma'}] &= i\hbar\delta_{\sigma\sigma'}\\
\text{(iv)}[h_\sigma, H_\gamma] &= 0\\
\text{(v)}[\pi_\sigma, \Pi_\gamma] &= 0\\
\text{(vi)}[h_\sigma, \Pi_\gamma] &= 0\\
\text{(vii)}[\pi_\sigma, H_\gamma] &= 0\\
\text{(viii)}[H_\gamma, H_{\gamma'}] &= 0\\
\text{(ix)}[\Pi_\gamma, \Pi_{\gamma'}] &= 0\\
\text{(x)}[H_\gamma, \Pi_{\gamma'}] &= i\hbar\delta_{\gamma\gamma'}.
\end{aligned} \tag{S.1.3}$$

It is straightforward to show that conditions (i-v), and condition (viii) are valid. For condition (vi), we can see that

$$\begin{aligned}
[h_\sigma, \Pi_\gamma] =& \frac{1}{N\bar{C}}\sum_{n,n',\sigma,\alpha,\beta}\chi^\gamma_{\alpha\beta}(r_{n,\sigma}p'_{n'\alpha}r'_{n'\beta} - p'_{n'\alpha}r'_{n'\beta}r_{n\sigma}) =\\
=& \frac{i\hbar}{N\bar{C}}\sum_{n,\alpha,\beta,\sigma} r'_{n\beta}\delta_{\alpha\sigma} = 0,
\end{aligned} \tag{S.1.4}$$

where we have that $\sum_n r'_{n,\beta} = 0$. The same reasoning can be used to show that condition (vii) is also trivially followed. For condition (ix) we find

$$\begin{aligned}[\Pi_\gamma, \Pi_{\gamma'}] =& \frac{1}{\bar{C}^2} \sum_{n,n',\alpha,\beta,\alpha',\beta'} \chi^\gamma_{\alpha\beta}\chi^{\gamma'}_{\alpha'\beta'}(p'_{n\alpha}r'_{n\beta}p'_{n'\alpha'}r'_{n'\beta'} - p'_{n'\alpha'}r'_{n\beta'}p'_{n'\alpha}r'_{n'\beta}) = \\ =& \frac{i\hbar}{\bar{C}^2} \sum_{\alpha,\beta,\alpha',\beta'} \chi^\gamma_{\alpha\beta}\chi^{\gamma'}_{\alpha'\beta'}(p'_{n\alpha}r'_{n'\beta'}\delta_{\alpha'\beta} - p'_{n\alpha'}r'_{n\beta}\delta_{\alpha\beta'}) \\ =& \frac{2i\hbar}{\bar{C}^2} \sum_{\alpha,\beta,\sigma} \left(\chi^\gamma_{\alpha\sigma}\chi^{\gamma'}_{\sigma\beta} - \chi^{\gamma'}_{\alpha\sigma}\chi^\gamma_{\sigma\beta}\right) \sum_n p'_{n\alpha}r'_{n\beta} = 0.\end{aligned} \tag{S.1.5}$$

For this to be met we impose that the matrices $\chi_\gamma$ are symmetric.

Condition (x) is written as

$$\begin{aligned}[H_\gamma, \Pi_{\gamma'}] =& \frac{1}{N\bar{C}^2} \sum_{n,n',\alpha,\beta,\alpha',\beta'} \chi^\gamma_{\alpha\beta}\chi^{\gamma'}_{\alpha'\beta'}(r'_{n\alpha}r'_{n\beta}p'_{n'\alpha'}r'_{n'\beta'} - p'_{n'\alpha'}r'_{n\beta'}r'_{n'\alpha}r'_{n'\beta}) = \\ =& \frac{i\hbar}{N\bar{C}^2} \sum_{\alpha,\beta,\alpha',\beta'} \chi^\gamma_{\alpha\beta}\chi^{\gamma'}_{\alpha'\beta'}(r'_{n\alpha}r'_{n'\beta'}\delta_{\alpha'\beta} + r'_{n\beta}r'_{n\beta'}\delta_{\alpha\alpha'}) \\ =& \frac{i\hbar}{N\bar{C}^2} \sum_{\alpha,\beta,\sigma} \left(\chi^\gamma_{\alpha\sigma}\chi^{\gamma'}_{\sigma\beta} + \chi^\gamma_{\sigma\beta}\chi^\gamma_{\sigma\beta'}\right) \sum_n r'_{n\alpha}r'_{n\beta}.\end{aligned} \tag{S.1.6}$$

We make use of the spherical symmetry of the particles and assume the charge displacements to be small compared to the total charge distribution. The sum in the dynamical variables $r'_{n\alpha}r'_{n\beta}$ can then be substituted by the expectation value $\langle r'_{n\alpha}r'_{n\beta}\rangle = 1/3\langle r^2_n\rangle\delta_{\alpha\beta}$.

$$\frac{1}{N}\sum_n r'_{n\alpha}r'_{n\alpha} \sim \frac{1}{3N}\sum_n \langle r^2_n\rangle \sim \frac{4\pi g}{3N}\int_0^\rho r^4 dr = \frac{4\pi g}{3N}\frac{\rho^5}{5} = \frac{\rho^2}{5}, \tag{S.1.7}$$

where we have used that $N \sim g4\pi\rho^3/3$. $g$ is the density of free electrons in the particle. By choosing these symmetric matrices

$$\chi_\gamma = \tfrac{1}{\sqrt{2}}\begin{pmatrix}1 & 0 & 0\\ 0 & -1 & 0\\ 0 & 0 & 0\end{pmatrix}, \; \tfrac{1}{\sqrt{6}}\begin{pmatrix}-1 & 0 & 0\\ 0 & -1 & 0\\ 0 & 0 & 2\end{pmatrix}, \; \tfrac{1}{\sqrt{2}}\begin{pmatrix}0 & 1 & 0\\ 1 & 0 & 0\\ 0 & 0 & 0\end{pmatrix}, \; \tfrac{1}{\sqrt{2}}\begin{pmatrix}0 & 0 & 0\\ 0 & 0 & 1\\ 0 & 1 & 0\end{pmatrix}, \; \tfrac{1}{\sqrt{2}}\begin{pmatrix}0 & 0 & 1\\ 0 & 0 & 0\\ 1 & 0 & 0\end{pmatrix}, \tag{S.1.8}$$

and considering $\bar{C} = \rho\sqrt{2/5}$ we obtain

$$[H_\gamma, \Pi_{\gamma'}] = \frac{2i\hbar}{N\bar{C}^2}\sum_{\alpha,\sigma}\chi^\gamma_{\alpha\sigma}\chi^{\gamma'}_{\sigma\alpha}\sum_n r'_{n\alpha}r'_{n\alpha} \sim i\hbar\delta_{\gamma\gamma'}. \tag{S.1.9}$$

In summary, all commutation relations are met approximately as long as the electronic displacement does not deviate too much from the original spherical distribution. The approximation is well suited for localized surface plasmons in metallic nanoparticles, because the charge distribution varies only along the surface of the particle. We should also mention that the assumption of symmetric $\chi$ matrices can only be applied if the total angular momentum of the electrons in the nanoparticle vanishes.

We now assume that the $\chi$ matrices together with the identity complete the space of relevant variables $H$. This means that any symmetric matrix $\bar{A}$ can be written as

$$A_{\alpha\beta} = a_0\delta_{\alpha\beta} + \sum_\gamma a_\gamma \chi^\gamma_{\alpha\beta}, \tag{S.1.10}$$

where $a_0$ and $a_\gamma$ are real values. We can then use the orthonormality of the $\chi_\gamma$ matrices to find

$$\sum_n \vec{r}_n\vec{r}_n = \sum_n r_{n\alpha}r_{n\beta} = N\rho^2\frac{2}{5}\left(1+\frac{5}{2}\frac{\vec{h}\cdot\vec{h}}{\rho^2}\right)\mathbf{1} + N\rho\sqrt{\frac{2}{5}}\sum_\gamma\left(H_\gamma + \frac{\sqrt{5/2}}{\rho}[\chi_\gamma : \vec{h}\vec{h}]\right)\chi_\gamma, \tag{S.1.11}$$

and

$$\sum_n \vec{p}_n\vec{r}_n = \sum_{n\alpha\beta} p_{n\alpha}r_{n\beta} = (\vec{h}\cdot\vec{h})\mathbf{1} + \rho\sqrt{\frac{2}{5}}\sum_\gamma\left(\Pi_\gamma + \frac{\sqrt{5/2}}{\rho}[\chi_\gamma : \vec{\pi}\vec{h}]\right)\chi_\gamma, \tag{S.1.12}$$

where $\mathbf{1}$ is the $3\times 3$ identity matrix.

Finally, we note that the terms depending on $\vec{h}\cdot\vec{h}$ and $\vec{h}\vec{h}$ will be small compared to the radius of the nanoparticle and can be neglected. As we will see below, they would also lead to higher-order interactions (involving three or more dynamical variables) and to non-quadratic Hamiltonians.

In summary, we found that within our approximation

$$\sum_n \vec{r}_n\vec{r}_n \sim N\bar{\rho}^2\left(\mathbf{1} + \frac{1}{\bar{\rho}}\sum_\gamma H_\gamma\chi_\gamma\right) \tag{S.1.13}$$

and

$$\sum_n \vec{p}_n\vec{r}_n \sim \bar{\rho}\sum_\gamma \Pi_\gamma\chi_\gamma, \tag{S.1.14}$$

where we have defined $\bar{\rho} = \sqrt{2/5}\rho$.

# 2 Light-Matter Interaction for Dipole and Quadrupole Excitations

In this section we show a general procedure for obtaining the Hamiltonian describing the interaction between light and a localized charge distribution in terms of the dipole and quadrupole moments. In principle, this could be further generalized to higher-order multipoles - provided that those could be written in terms of conjugate coordinates and momenta. This will be applied for each individual particle at position $\vec{R}$. The extension to other particles is trivial as long as there is no exchange of charges between the different particles.

We start with the Hamiltonian for a set of charges distributed in space, given by

$$\mathcal{H} = \sum_n \frac{1}{2m}\left[\vec{p}_n - \mathrm{q}_n\vec{A}(\vec{r}_n,t)\right]^2 + \mathcal{H}_{Coul} + \mathcal{H}_L, \tag{S.2.1}$$

where $\mathcal{H}_{Coul}$ is the Coulomb interaction between the different $n$ charges in the system, $\mathcal{H}_L$ is the quantized free-electromagnetic field Hamiltonian and $\vec{p}_n$ is the conjugate momentum to $\vec{r}_n$. We rewrite this Hamiltonian in terms of the new set of canonical variables introduced in Sec. 1. Thereby, the matter Hamiltonian

$$\mathcal{H}_M = \sum_n \frac{p_n^2}{2m} + \mathcal{H}_{Coul}, \tag{S.2.2}$$

becomes

$$\mathcal{H}_M = \mathcal{H}_M^D + \mathcal{H}_M^Q + \mathcal{H}_M^{HO} + \mathcal{H}_{\text{plpl}}, \tag{S.2.3}$$

where $\mathcal{H}_M^D$+ $\mathcal{H}_M^Q$ describe the dynamics for the dipole-like and quadrupole-like canonical variables of each individual particle. $\mathcal{H}_{\text{plpl}}$ respresents the interaction between plasmonic excitations in different particles. The term $\mathcal{H}_M^{HO}$ represents the dynamics of the higher-order coordinates, which, within our present model, will be disregarded.

The Hamiltonian for the quantized electromagnetic field remains unchanged. We therefore turn our attention in the following to the light-matter interaction Hamiltonian.

## 2.1 Taylor's Series Expansion

When the electronic charge is closely localized in a small region, such as in a metallic nanoparticle, it is usual to expand the vector potential in a Taylor series and retain the lower order contributions. With this, the light-matter interaction will be separated into four parts $\mathcal{H}_{LM}^{(D,1)}$, $\mathcal{H}_{LM}^{(D,2)}$, $\mathcal{H}_{LM}^{(Q,1)}$ and $\mathcal{H}_{LM}^{(Q,2)}$. The first (last) two terms correspond to the first- and second-order contributions of the dipole (quadrupole) plasmonic excitations of the nanoparticles. The first-order dipole and quadrupole terms are

$$\mathcal{H}_{LM}^{(D,1)} = -\frac{\mathrm{q}}{m}\sum_n \vec{p}_n \cdot \vec{A}(\vec{R}) \rightarrow -\frac{\mathrm{Q}}{M}\vec{\pi} \cdot \vec{A}(\vec{R}), \tag{S.2.4}$$

and

$$\mathcal{H}_{LM}^{(Q,1)} = -\frac{\mathrm{q}}{m}\sum_n \vec{p}_n \cdot \nabla_n \vec{A}(\vec{R}) \cdot \vec{r}_n \rightarrow -\frac{\mathrm{Q}\bar{\rho}}{M}\sum_\gamma [\Pi_\gamma : \nabla \vec{A}(\vec{R})], \tag{S.2.5}$$

where we have used the definition of the dipole momentum $\vec{\pi}$ in Eq.(S.1.2) and also Eq. (S.1.14) for defining $\Pi_\gamma$. $\nabla \vec{A}(\vec{R}) = \frac{\partial}{\partial \alpha} A_\beta \hat{e}_\alpha \hat{e}_\beta$ is a dyadic gradient of the vector potential. For the second-order interaction, the dipole contribution is given by

$$\mathcal{H}_{LM}^{(D,2)} = \frac{\mathrm{Q}^2}{M}\vec{A}^\dagger(\vec{R}) \cdot \vec{A}(\vec{R}), \tag{S.2.6}$$

while the quadrupole term is given by

$$\begin{aligned}\mathcal{H}_{LM}^{(Q,2)} = \frac{\mathrm{q}^2}{m}\sum_n \vec{r}_n \cdot \nabla \vec{A}^\dagger(\vec{R}) \cdot \nabla \vec{A}(\vec{R}) \cdot \vec{r}_n \rightarrow & \frac{\mathrm{q}^2}{m}[\sum_n \vec{r}_n \vec{r}_n : (\nabla \vec{A}^\dagger \cdot \nabla \vec{A})_{\vec{R}}] = \\ = & \frac{\mathrm{Q}^2 \bar{\rho}^2}{2M}[\mathbf{1} + \frac{1}{\bar{\rho}_j}\sum_\gamma H_\gamma \chi_\gamma] : (\nabla \vec{A}^\dagger \cdot \nabla \vec{A})_{\vec{R}},\end{aligned} \tag{S.2.7}$$

where we have used Eq. (S.1.13).

The second term on the right-hand side depends on three dynamical variables, corresponding to a non-quadratic term in the Hamiltonian. This term will be disregarded and the second-order light-quadrupole interaction term is reduced to

$$\mathcal{H}_{LM}^{(Q,2)} = \frac{\mathrm{Q}^2\bar{\rho}^2}{2M}[\mathbf{1} : (\nabla\vec{A}^\dagger \cdot \nabla\vec{A})_{\vec{R}}] = \frac{\mathrm{Q}^2\bar{\rho}^2}{2M}[\nabla\vec{A}^\dagger \cdot (\nabla\vec{A})^T]_{\vec{R}}, \tag{S.2.8}$$

where we have used the properties of the double dot product. $(T)$ stands here for the transpose of the dyadic $\nabla\vec{A}(R)$. It should also be noted that another term appears in the expansion of $\mathcal{H}_{LM}$,

$$\frac{\mathrm{q}^2}{m}\sum_n \vec{A}(\vec{R}) \cdot \nabla\vec{A}(\vec{R}) \cdot \vec{r}_n \to \frac{\mathrm{Q}^2}{M}\vec{A}(\vec{R}) \cdot \nabla\vec{A}(\vec{R}) \cdot \vec{h}. \tag{S.2.9}$$

This term is also third-order and is therefore disregarded in our analysis.

We now apply this to a spherical charge distribution, localized around a position $\vec{R}$, that is interacting with the electromagnetic (EM) field. We can write the EM field in the Coulomb gauge as

$$\vec{A}(\vec{R}+\vec{r}) = \sum_{\vec{q},\lambda} A_{\vec{q},\lambda} e^{i\vec{q}\cdot(\vec{r}+\vec{R})} = \sum_{\vec{q}} \vec{A}_{\vec{q},\vec{R}} \exp(i\vec{q}\cdot\vec{r}), \tag{S.2.10}$$

where $\vec{A}_{\vec{q},\vec{R}} = A_{\vec{q}} \exp(i\vec{q}\cdot\vec{R})$. The gradient of the EM field can be written in a dyadic form as $\nabla\vec{A}(\vec{R}) = i\vec{q}\vec{A}_{\vec{q},\vec{R}}$ and the quadrupole contributions to the light-matter interaction become

$$\mathcal{H}_{LM}^{(Q,1)} = -i\frac{\mathrm{Q}\bar{\rho}}{M}\sum_{\vec{q}\gamma} \Pi_\gamma : \vec{q}\vec{A}_{\vec{q},\vec{R}}, \tag{S.2.11}$$

and

$$\mathcal{H}_{LM}^{(Q,2)} = \frac{\mathrm{Q}^2\bar{\rho}^2}{2M}\sum_{\vec{q},\vec{q}'} \vec{A}_{\vec{q}',\vec{R}}\vec{q}' \cdot \vec{q}\vec{A}_{\vec{q},\vec{R}}. \tag{S.2.12}$$

## 2.2 Spherical Harmonics Expansion

If the nanoparticle radius is a considerable fraction of the light wavelength, the Taylor expansion will not converge fast enough and higher-order contributions would need to be taken into account. Alternatively, for spherical nanoparticles it is reasonable to expand the plane wave part of the vector potential into spherical harmonics

$$\exp(i\vec{q}\cdot\vec{r}) = 4\pi\sum_{l,m} i^l j_l(qr) Y_{lm}^*(\hat{k}) Y_{lm}(\hat{r}), \tag{S.2.13}$$

where $j_l$ are the spherical Bessel functions and $Y_{lm}$ the spherical harmonics. This can be written as

$$\begin{aligned}\exp(i\vec{q}\cdot\vec{r}) =& j_0(qr) + 3ij_1(qr)\Bigg(\cos(\theta_r)\cos(\theta_k) + \\ &+\frac{1}{2}\sin(\theta_k)\sin(\theta_r)e^{i(\phi_r-\phi_k)} + \frac{1}{2}\sin(\theta_k)\sin(\theta_r)e^{-i(\phi_r-\phi_k)}\Bigg) + \mathrm{H.O.},\end{aligned} \tag{S.2.14}$$

where H.O. refers to the higher-order terms. Disregarding the higher-order terms, we have

$$\exp(i\vec{q}\cdot\vec{r}) \sim j_0(qr) + 3ij_1(qr)\hat{q}\cdot\hat{r}. \tag{S.2.15}$$

We now apply this expansion to the first-order part of the light-matter interaction

$$\begin{aligned}\mathcal{H}^{(1)}_{LM} &= -\frac{\mathrm{q_e}}{m_e}\sum_{n,\vec{q},\lambda}\vec{p}_{n,\lambda}A_{\vec{q},\vec{R},\lambda}\exp[i\vec{q}\cdot(\vec{r}_n)] \\ &\sim -\frac{\mathrm{q_e}}{m_e}\sum_{n,\vec{q},\lambda}\vec{p}_{n,\lambda}A_{\vec{q},\vec{R},\lambda}\left(j_0(qr_n) + \frac{3j_1(qr_n)}{qr_n}i\vec{q}\cdot\vec{r}_n\right).\end{aligned} \tag{S.2.16}$$

This can be separated in two terms: the dipole term is given by

$$\mathcal{H}^{(D,1)}_{LM} = -\frac{\mathrm{q_e}}{m_e}\sum_{\lambda,\vec{q}}A_{\vec{q},\vec{R},\lambda}\sum_n p_{n\lambda}j_0(qr_n), \tag{S.2.17}$$

and the quadrupole term is

$$\mathcal{H}^{(Q,1)}_{LM} = -\frac{\mathrm{q_e}}{m_e}\sum_{\lambda,\vec{q},\alpha,\beta} iqA_{\vec{q},\vec{R},\lambda}\left(\hat{e}_\lambda\hat{e}_q : \hat{e}_\alpha\hat{e}_\beta\right)\sum_n\frac{3j_1(qr_n)}{qr_n}p_{n\alpha}r_{n\beta}. \tag{S.2.18}$$

As an approximation, we can exchange the functions $j_0(qr_n)$ and $3j_1(qr_n)/qr_n$ by their mean value inside the particle, given by

$$\mathrm{f}_D(q\rho) = \langle j_0(qr)\rangle = \frac{1}{4\pi\rho^3/3}4\pi\int_0^\rho dr j_0(qr)r^2 = \frac{3}{(q\rho)^3}\left[\sin(q\rho) - q\rho\cos(q\rho)\right], \tag{S.2.19}$$

and

$$\mathrm{f}_Q(q\rho) = \langle\frac{3j_1(qr_n)}{qr_n}\rangle = \frac{1}{4\pi\rho^3/3}4\pi\int_0^\rho dr\frac{3j_1(qr)}{qr}r^2 = \frac{9}{(q\rho)^3}\left[\mathrm{Si}(q\rho) - \sin(q\rho)\right], \tag{S.2.20}$$

where $\mathrm{Si}(x)$ is the sine integral function.

Applying the same procedure as in the previous section, the first-order light-matter interaction is

$$\mathcal{H}^{(D,1)}_{LM} = -\frac{\mathrm{Q}}{M}\sum_{\vec{q}}\mathrm{f}_D(q\rho)\vec{\pi}\cdot\vec{A}_{\vec{q},\vec{R}}, \tag{S.2.21}$$

and

$$\mathcal{H}^{(Q,1)}_{LM} = -i\frac{\mathrm{Q}\bar{\rho}}{M}\sum_{\gamma\lambda,\vec{q}}\mathrm{f}_Q(q\rho)\Pi_\gamma : \vec{q}\vec{A}_{\vec{q},\vec{R}}. \tag{S.2.22}$$

Finally, the second-order terms are

$$\mathcal{H}^{(D,2)}_{LM} = -\frac{\mathrm{Q}}{M}\sum_{\vec{q}\vec{q}'}\mathrm{f}_D(q'\rho)\mathrm{f}_D(q\rho)\vec{A}_{\vec{q}',\vec{R}}\cdot\vec{A}_{\vec{q},\vec{R}}, \tag{S.2.23}$$

and

$$\mathcal{H}^{(Q,2)}_{LM} = \frac{\mathrm{Q}^2\bar{\rho}^2}{2M}\sum_{\vec{q}\vec{q}'}\mathrm{f}_D(q'\rho)\mathrm{f}_D(q\rho)[\vec{A}_{\vec{q},\vec{R}}\vec{q}'\cdot\vec{q}\vec{A}_{\vec{q},\vec{R}}]. \tag{S.2.24}$$

Here we also disregarded non-quadratic terms.

# 3 Nanoparticle Supercrystals

We now consider a system composed of a set of different particles. The excitations of the charge distribution can be written in terms of plasmon oscillations of each of the individual particles, their mutual interaction and their interaction with the electromagnetic field. Furthermore, we assume that the particles are arranged in a crystalline structure such that each particle is characterized by a lattice vector $\vec{R}$ and an index $j$.

## 3.1 Plasmon-Plasmon Interaction

For both the dipole and quadrupole canonical variables, we propose that the effective Coulomb interaction within each particle acts on these variables as a harmonic potential, such that

$$\mathcal{H}_M^D = \sum_{\vec{R},j,\sigma} \frac{\pi^2_{\vec{R},j,\sigma}}{2M_j} + \frac{M_j \omega^2_{D,j}}{2} h^2_{\vec{R},j,\sigma}, \tag{S.3.1}$$

and

$$\mathcal{H}_M^Q = \sum_{\vec{R},j,\gamma} \frac{\Pi^2_{\vec{R},j,\gamma}}{2M_j} + \frac{M_j \omega^2_{Q,j}}{2} H^2_{\vec{R},j,\gamma}. \tag{S.3.2}$$

Now, we define

$$\begin{cases} h_{\vec{R},j,\sigma} = \sqrt{\frac{\hbar}{2M_j\omega_j^D}}(b^\dagger_{\vec{R},j,\sigma} + b_{\vec{R},j,\sigma}) \\ \pi_{\vec{R},j,\sigma} = \sqrt{\frac{\hbar M_j \omega_j^D}{2}}(b^\dagger_{\vec{R},j,\sigma} - b_{\vec{R},j,\sigma}) \end{cases} \tag{S.3.3}$$

$$\begin{cases} H_{\vec{R},j,\gamma} = \sqrt{\frac{\hbar}{2M_j\omega_{Qj}}}(b^\dagger_{\vec{R},j,\gamma} + b_{\vec{R},j,\gamma}) \\ \Pi_{\vec{R},j,\gamma} = \sqrt{\frac{\hbar M_j \omega_{Q,j}}{2}}(b^\dagger_{\vec{R},j,\gamma} - b_{\vec{R},j,\gamma}) \end{cases} \tag{S.3.4}$$

With this, we have

$$\mathcal{H}_M^D = \sum_{\vec{R},j,\sigma} \left(b^\dagger_{\vec{R},j,\sigma} b_{\vec{R},j,\sigma} + 1/2\right) \hbar\omega_{D,j}, \tag{S.3.5}$$

and

$$\mathcal{H}_M^Q = \sum_{\vec{R},j,\gamma} \left(b^\dagger_{\vec{R},j,\gamma} b_{\vec{R},j,\gamma} + 1/2\right) \hbar\omega_{Q,j}. \tag{S.3.6}$$

We can associate each of these canonical variables $h$ and $H$ with dipole and quadrupole moments

$$\vec{\mathrm{p}} = \sum_{\sigma} \mathrm{Q}_{D,j} h_{\vec{R},j,\sigma} \hat{e}_\sigma, \tag{S.3.7}$$

and

$$\bar{\mathcal{Q}} = \sum_{\gamma} \mathrm{Q}_{Q,j} \bar{\rho}_j H_{\vec{R},j,\gamma} \chi_\gamma, \tag{S.3.8}$$

where $\mathrm{Q}_{D,j}$ and $\mathrm{Q}_{Q,j}$ are the screened dipole and quadrupole effective charges for each particle $j$.

The plasmon-plasmon interaction can now be written as

$$\mathcal{H}_{\text{plpl}} = 1/2 \sum_{\vec{R},\vec{R}'} \mathcal{H}_{\text{DD}}(\vec{R},\vec{R}') + \mathcal{H}_{\text{DQ}}(\vec{R},\vec{R}') + \mathcal{H}_{\text{QQ}}(\vec{R},\vec{R}') + ... \tag{S.3.9}$$

where $DD$ represents the dipole-dipole interaction, $DQ$ is for the dipole-quadrupole interaction, and $QQ$ is for the quadrupole-quadrupole interaction.

### 3.1.1 Dipole-Dipole Interaction

The interaction between two dipoles at lattice sites $\vec{R}_j$ and $\vec{R}'_{j'}$ can be described by

$$\mathcal{H}_{\text{DD}}(\vec{R}_j,\vec{R}'_{j'}) = \frac{1}{4\pi\epsilon_0\epsilon_m}\frac{\vec{\mathrm{p}}\cdot\vec{\mathrm{p}}' - 3(\vec{\mathrm{p}}\cdot\vec{n})(\vec{\mathrm{p}}'\cdot\vec{n})}{|\vec{R}_j - \vec{R}'_{j'}|^3}, \tag{S.3.10}$$

where $\epsilon_m$ is the dielectric constant of the surrounding medium.

It is convenient to define the Fourier transform of the ladder operators as

$$b_{\vec{R},j,\sigma} = \frac{1}{\sqrt{N}}\sum_{\vec{q}} b_{\vec{q},j,\sigma} \exp i\vec{q}\cdot\vec{R}_j, \tag{S.3.11}$$

where $N$ is the number of unit cells in the supercrystal and $\vec{q}$ is restricted to the first Brillouin zone. With this Fourier transformation $\mathcal{H}_M^D$ becomes

$$\mathcal{H}_M^D = \sum_{\vec{q},j,\sigma}\left(b^{\dagger}_{\vec{q},j,\sigma}b_{\vec{q},j,\sigma} + 1/2\right)\hbar\omega_j^D. \tag{S.3.12}$$

Defining

$$\vec{n}_{j,j'} = \frac{\vec{R}_{jj'}}{|\vec{R}_{jj'}|} = \frac{\vec{R}_j - \vec{R}'_j}{|\vec{R}_j - \vec{R}'_j|}, \tag{S.3.13}$$

the dipole-dipole part of the plasmon-plasmon interaction becomes

$$\begin{aligned}
\mathcal{H}_{\rm DD} =& \frac{1}{2}\sum_{\vec{R}_j,R'_{j'},\sigma,\sigma'} \frac{\mathrm{Q}_j^D \mathrm{Q}_j^D}{4\pi\epsilon_0\epsilon_m} \\
&\times \frac{h_{\vec{R},j,\sigma} h_{\vec{R}'j'\sigma'}\delta_{\sigma\sigma'} - 3(h_{\vec{R}j\sigma}\hat{e}_\sigma\cdot\vec{n}_{jj'})(h_{\vec{R}'j'\sigma'}\hat{e}_{\sigma'}\cdot\vec{n}_{jj'})}{|\vec{R}_j-\vec{R}'_{j'}|^3} \\
=& \frac{1}{2}\sum_{\vec{R},j,j',\vec{q},\vec{q}',\sigma,\sigma'} \frac{\mathrm{Q}_j^D}{\sqrt{2M_j\omega_j^D}} \frac{\mathrm{Q}_{j'}^D}{\sqrt{2M_{j'}\omega_{j',\sigma'}}} \frac{\hbar}{4\pi\epsilon_m\epsilon_0} \\
&\times \frac{\delta_{\sigma\sigma'} - 3(\hat{e}_\sigma\cdot\vec{n}_{jj'})(\hat{e}_{\sigma'}\cdot\vec{n}_{jj'})}{|\vec{R}_{jj'}|^3} \\
&\times \Big[ b^\dagger_{\vec{q},j,\sigma} b^\dagger_{\vec{q}',j',\sigma'} e^{-i(\vec{q}\cdot\vec{R}_j+\vec{q}'\cdot\vec{R}_{j'})} + b^\dagger_{\vec{q},j,\sigma} b_{\vec{q}',j',\sigma'} e^{-i(\vec{q}\cdot\vec{R}_j-\vec{q}'\cdot\vec{R}_{j'})} + \\
&\quad + b_{\vec{q},j,\sigma} b^\dagger_{\vec{q}',j',\sigma'} e^{i(\vec{q}\cdot\vec{R}_j-\vec{q}'\cdot\vec{R}_{j'})} + b_{\vec{q},j,\sigma} b_{\vec{q}',j',\sigma'} e^{i(\vec{q}\cdot\vec{R}_j+\vec{q}'\cdot\vec{R}_{j'})} \Big] \\
=& \frac{1}{2}\sum_{\vec{R},j,j',\vec{q},\vec{q}',\sigma,\sigma'} \frac{\mathrm{Q}_j^D}{\sqrt{2M_j\omega_j^D}} \frac{\mathrm{Q}_{j'}^D}{\sqrt{2M_{j'}\omega_{j',\sigma'}}} \frac{\hbar}{4\pi\epsilon_m\epsilon_0} \\
&\times \frac{\delta_{\sigma\sigma'} - 3(\hat{e}_\sigma\cdot\vec{n}_{jj'})(\hat{e}_{\sigma'}\cdot\vec{n}_{jj'})}{|\vec{R}_{jj'}|^3} \\
&\times \Big[ b^\dagger_{\vec{q},j,\sigma} b^\dagger_{\vec{q}',j',\sigma'} e^{-i(\vec{q}+\vec{q}')\cdot\vec{R}_j} e^{i\vec{q}'\cdot\vec{R}_{jj'}} + b^\dagger_{\vec{q},j,\sigma} b_{\vec{q}',j',\sigma'} e^{-i(\vec{q}-\vec{q}')\cdot\vec{R}_j} e^{-i\vec{q}'\cdot\vec{R}_{jj'}} + \\
&\quad + b_{\vec{q},j,\sigma} b^\dagger_{\vec{q}',j',\sigma'} e^{i(\vec{q}-\vec{q}')\cdot\vec{R}_j} e^{-i\vec{q}'\cdot\vec{R}_{jj'}} + b_{\vec{q},j,\sigma} b_{\vec{q}',j',\sigma'} e^{i(\vec{q}+\vec{q}')\cdot\vec{R}_j} e^{i\vec{q}'\cdot\vec{R}_{jj'}} \Big] \\
=& \frac{1}{2}\sum_{\vec{R},j,j',\vec{q},\sigma,\sigma'} \frac{\mathrm{Q}_j^D}{\sqrt{2M_j\omega_j^D}} \frac{\mathrm{Q}_{j'}^D}{\sqrt{2M_{j'}\omega_{j'}^D}} \frac{\hbar}{4\pi\epsilon_m\epsilon_0} \\
&\times \frac{\delta_{\sigma\sigma'} - 3(\hat{e}_\sigma\cdot\vec{n}_{jj'})(\hat{e}_{\sigma'}\cdot\vec{n}_{jj'})}{|\vec{R}_{jj'}|^3} \\
&\times \Big[ b^\dagger_{\vec{q},j,\sigma} b^\dagger_{-\vec{q},j',\sigma'} e^{-i\vec{q}\cdot\vec{R}_{jj'}} + b^\dagger_{\vec{q},j,\sigma} b_{\vec{q},j',\sigma'} e^{-i\vec{q}\cdot\vec{R}_{jj'}} + \\
&\quad + b_{\vec{q},j,\sigma} b^\dagger_{\vec{q},j',\sigma'} e^{-i\vec{q}\cdot\vec{R}_{jj'}} + b_{\vec{q},j,\sigma} b_{-\vec{q},j',\sigma'} e^{-i\vec{q}\cdot\vec{R}_{jj'}} \Big].
\end{aligned} \tag{S.3.14}$$

where we have used $\sum_j \exp[i(\vec{q}\mp\vec{q}')\cdot\vec{R}_j]/N = \delta_{\vec{q}',\pm\vec{q}}$. With these considerations, the plasmon-plasmon interaction takes the form

$$\begin{aligned}
\mathcal{H}_{\rm plpl} =& \sum_{\vec{R},j,j',\vec{q},\sigma,\sigma'} \sqrt{\frac{\hbar(\mathrm{Q}_j^d)^2}{8\pi\epsilon_0\epsilon_m M_j\omega_j^D}} \sqrt{\frac{\hbar(\mathrm{Q}_{j'}^d)^2}{8\pi\epsilon_0\epsilon_m M'_j\omega_{j',\sigma'}}} \\
&\times \frac{1}{2}\frac{\delta_{\sigma\sigma'} - 3(\hat{e}_\lambda\cdot\vec{n}_{jj'})(\hat{e}_{\sigma'}\cdot\vec{n}_{jj'})}{|\vec{R}_{jj'}|^3} \exp(i\vec{q}\cdot\vec{R}_{jj'}) \\
&\times \Big[ b^\dagger_{\vec{-}q,j,\sigma} b^\dagger_{\vec{q},j',\sigma'} + b^\dagger_{\vec{-}q,j,\sigma} b_{\vec{-}q,j',\sigma'} + b_{\vec{q},j,\sigma} b^\dagger_{\vec{q},j',\sigma'} + b_{\vec{q},j,\sigma} b_{-\vec{q},j',\sigma'} \Big].
\end{aligned} \tag{S.3.15}$$

For this last step we rearranged selected $\vec{q}$ and $-\vec{q}$ terms in the sum.

Now, to have a scaleless structure factor $S$, we can divide all distances by $\overline{R} = (V_{\rm uc})^{1/3}$, leading to

$$S^{DD}_{j\sigma,j'\sigma'}(\vec{q}) = \sum_{\vec{R}} \frac{1}{2}\frac{\delta_{\sigma\sigma'} - 3(\hat{e}_\sigma\cdot\vec{n}_{jj'})(\hat{e}_{\sigma'}\cdot\vec{n}_{jj'})}{|\vec{R}_{jj'}/\overline{R}|^3} \exp(i\vec{q}\cdot\vec{R}_{jj'}). \tag{S.3.16}$$

With this, we can define the coupling tensor for the dipole as

$$\Lambda_{D,j} = \frac{(\mathrm{Q}_j^D)^2}{8\pi\epsilon_0\epsilon_m M_j\omega_j V_{uc}}. \tag{S.3.17}$$

The dipole-dipole interaction now has the form

$$\mathcal{H}_{\mathrm{DD}} = \sum_{j,j',\vec{q},\sigma,\sigma'} \hbar\sqrt{\Lambda_{D,j}\Lambda_{D,j'}} S^{DD}_{j\sigma,j'\sigma'}(\vec{q}) \left(b^\dagger_{-\vec{q},j,\sigma} + b_{\vec{q},j',\sigma'}\right)\left(b_{-\vec{q},j',\sigma'} + b^\dagger_{\vec{q},j,\sigma}\right). \tag{S.3.18}$$

### 3.1.2 Quadrupole-Quadrupole Interaction

The interaction between two quadrupoles with different moments separated by the vector $\vec{r}$ is

$$\mathcal{H}_{QQ} = \frac{1}{4\pi\epsilon_0\epsilon_m}\frac{1}{3r^5}\left\{35(\mathcal{Q} : \hat{e}_r\hat{e}_r)(\mathcal{Q}' : \hat{e}_r\hat{e}_r) - 20(\mathcal{Q}\mathcal{Q}' : \hat{e}_r\hat{e}_r) + 2(\mathcal{Q} : \mathcal{Q}')\right\}, \tag{S.3.19}$$

Substituting the equations for the quadrupole moments, we get

$$\begin{aligned}\mathcal{H}_{QQ} = \frac{1}{4\pi\epsilon_0\epsilon_m}\sum_{\vec{R}\vec{R}'jj'\gamma\gamma'}\frac{1}{6}\Bigg\{&35\frac{(\chi_\gamma : \hat{n}_{j,j'}\hat{n}_{j,j'})(\chi_{\gamma'} : \hat{n}_{j,j'}\hat{n}_{j,j'})}{R^5_{j,j'}} - 20\frac{(\chi_\gamma\chi_{\gamma'} : \hat{n}_{j,j'}\hat{n}_{j,j'})}{R^5_{j,j'}}\\ &+2\frac{(\chi_\gamma : \chi_{\gamma'})}{R^5_{j,j'}}\Bigg\} \times \mathrm{Q}_j^Q\bar{\rho}_j\mathrm{Q}_{j'}^Q\bar{\rho}_{j'}H_{\vec{R},j,\gamma}H_{\vec{R}',j',\gamma'}\end{aligned} \tag{S.3.20}$$

leading to

$$\begin{aligned}\mathcal{H}_{QQ} =& \frac{1}{4\pi\epsilon_0\epsilon_m}\sum_{\vec{R}\vec{R}'jj'\gamma\gamma'}\frac{1}{6}\Bigg\{35\frac{(\chi_\gamma : \hat{n}_{j,j'}\hat{n}_{j,j'})(\chi_{\gamma'} : \hat{n}_{j,j'}\hat{n}_{j,j'})}{R^5_{j,j'}} - 20\frac{(\chi_\gamma\chi_{\gamma'} : \hat{n}_{j,j'}\hat{n}_{j,j'})}{R^5_{j,j'}}\\ &+2\frac{(\chi_\gamma : \chi_{\gamma'})}{R^5_{j,j'}}\Bigg\}\sqrt{\frac{\hbar}{2M_j\omega_j^D}\frac{\hbar}{2M_{j'}\omega_{j'}^Q}}\mathrm{Q}_j^Q\bar{\rho}_j\mathrm{Q}_{j'}^Q\bar{\rho}_{j'}\times\\ &\times(b^\dagger_{\vec{q},j,\gamma}e^{i\vec{q}\cdot\vec{R}} + b_{-\vec{q},j,\gamma}e^{-i\vec{q}\cdot\vec{R}})(b^\dagger_{\vec{q},j',\gamma'}e^{i\vec{q}\cdot\vec{R}'} + b_{-\vec{q}',j',\gamma'}e^{-i\vec{q}'\cdot\vec{R}'}).\end{aligned} \tag{S.3.21}$$

We can then define the quadrupole coupling tensor

$$\Lambda_{Q,j} = \frac{(\mathrm{Q}_j^Q\bar{\rho}_j)^2}{8\pi\epsilon_0\epsilon_m M_j\omega_j^D V_{uc}^{5/3}}, \tag{S.3.22}$$

and the quadrupole-quadrupole structure function $S$ as

$$S^{QQ}_{j\gamma,j'\gamma'}(\vec{q}) = \sum_{\vec{R}}\frac{1}{6}\left\{35\frac{(\chi_\gamma : \hat{n}_{jj'}\hat{n}_{jj'})(\chi_{\gamma'} : \hat{n}_{jj'}\hat{n}_{jj'})}{(R_{jj'}/\bar{R})^5} - 20\frac{(\chi_\gamma\chi_{\gamma'} : \hat{n}_{jj'}\hat{n}_{jj'})}{(R_{jj'}/\bar{R})^5} + 2\frac{(\chi_\gamma : \chi_{\gamma'})}{(R_{j,j'}/\bar{R})^5}\right\}\exp(i\vec{q}\cdot\vec{R}_{jj'}), \tag{S.3.23}$$

such that the quadrupole-quadrupole interaction has the same shape as that of the dipole-dipole interaction:

$$H^{QQ}_{\mathrm{plpl}} = \sum_{\vec{R},j,j',\vec{q},\gamma,\gamma1}\hbar\sqrt{\Lambda_{Q,j}\Lambda_{Q,j'}}S^{QQ}_{j\gamma,j'\gamma'}(\vec{q})\left(b^\dagger_{-q,j,\gamma} + b_{\vec{q},j',\gamma'}\right)\left(b_{-\vec{q},j',\gamma'} + b^\dagger_{\vec{q},j,\gamma}\right). \tag{S.3.24}$$

### 3.1.3 Dipole-Quadrupole Interaction

Finally, the dipole-quadrupole interaction potential is

$$H^0_{DQ} = -5\left(\mathcal{Q} : \frac{\hat{e}_r\hat{e}_r}{r^4}\right)(\hat{e}_r \cdot \vec{\mathrm{p}}) + 2\left(\mathcal{Q} : \frac{\hat{e}_r\hat{e}_{\mathrm{p}}}{r^4}\right)\mathrm{p}. \tag{S.3.25}$$

The equation for the full dipole-quadrupole interaction in the 3D system can then be written as

$$\mathcal{H}_{DQ} = \sum_{\vec{R}\vec{R}'jj'\sigma\gamma} \frac{1}{2}\left[-5\left(\chi_\gamma : \frac{\hat{n}_{j,j'}\hat{n}_{j,j'}}{R^4_{j,j'}}\right)(\hat{n}_{j,j'} \cdot \hat{e}_\sigma) + 2\left(\chi_\gamma : \frac{\hat{n}_{j,j'}\hat{e}_\sigma}{R^4_{j,j'}}\right)\right] \mathrm{Q}^D_j \mathrm{Q}^Q_{j'} \bar{\rho}_{j'} h_{\vec{R},j,\sigma} H_{\vec{R}',j',\gamma}. \tag{S.3.26}$$

Again, we expand the dynamical variables in terms of the creation and annihilation operators for the lattice dipoles and quadrupoles

$$\begin{aligned} \mathcal{H}_{DQ} = &\frac{1}{4\pi\epsilon_0\epsilon_m} \sum_{\vec{R}\vec{R}'jj'\sigma\gamma} \sqrt{\frac{\hbar}{2M_j\omega^D_j}\frac{\hbar}{2M_{j'}\omega^Q_{j'}}} \mathrm{Q}^D_j \mathrm{Q}^Q_{j'} \bar{\rho}_{j'} \\ &\times \frac{1}{2}\left[-5\left(\chi_\gamma : \frac{\hat{n}_{j,j'}\hat{n}_{j,j'}}{R^4_{j,j'}}\right)(\hat{n}_{j,j'} \cdot \hat{e}_\sigma) + 2\left(\chi_\gamma : \frac{\hat{n}_{j,j'}\hat{e}_\sigma}{R^4_{j,j'}}\right)\right] \\ &\times (b^\dagger_{\vec{q},j,\sigma} e^{i\vec{q}\cdot\vec{R}} + b_{-\vec{q},j,\sigma} e^{-i\vec{q}\cdot\vec{R}})(b^\dagger_{\vec{q},j',\sigma'} e^{i\vec{q}\cdot\vec{R}'} + b_{-\vec{q}',j',\sigma'} e^{-i\vec{q}'\cdot\vec{R}'}). \end{aligned} \tag{S.3.27}$$

A direct comparison with the equation for the dipole-dipole interaction leads to a similar equation

$$H^{DQ}_{\mathrm{plpl}} = \sum_{\vec{R},j,j',\vec{q},\sigma,\gamma} \hbar\sqrt{\Lambda_{D,j}\Lambda_{Q,j'}} S^{DQ}_{j\sigma,j'\gamma}(\vec{q}) \left(b^\dagger_{-\vec{q},j,\sigma} + b_{\vec{q},j',\sigma'}\right)\left(b_{-\vec{q},j',\gamma} + b^\dagger_{\vec{q},j,\gamma}\right), \tag{S.3.28}$$

where the structure function $S$ is

$$S^{DQ}_{j\lambda,j'\gamma}(\vec{q}) = \sum_{\vec{R}} \frac{1}{2}\left[-5\left(\chi_\gamma : \frac{\hat{n}_{jj'}\hat{n}_{jj'}}{(R_{jj'}/\bar{R})^4}\right)(\hat{n}_{jj'} \cdot \hat{e}_\sigma) + 2\left(\chi_\gamma : \frac{\hat{n}_{jj'}\hat{e}_\sigma}{(R_{jj'}/\bar{R})^4}\right)\right] \exp(i\vec{q}\cdot\vec{R}_{jj'}). \tag{S.3.29}$$

### 3.1.4 General Plasmon-Plasmon Interaction

The similarities between the equations for the $DD$, $DQ$ and $QQ$ plasmon-plasmon interactions can be used to cast them into a general form

$$\mathcal{H}_{\mathrm{plpl}} = \sum_{\nu,\nu',\vec{q}} \hbar\sqrt{\Lambda_{\bar{\nu}}\Lambda_{\bar{\nu}'}} S^{\bar{\nu}\bar{\nu}'}_{\nu\nu'}(\vec{q}) \left(b^\dagger_{-\vec{q},\nu} + b_{\vec{q},\nu}\right)\left(b_{-\vec{q},\nu'} + b^\dagger_{\vec{q},\nu'}\right), \tag{S.3.30}$$

where $\nu \to j\sigma, j\gamma$ concatenates the labels for the 3 dipole and 5 quadrupole modes for each nanoparticle $j$ in the unit cell and $\bar{\nu} = D$ or $Q$ depending on whether $\nu$ corresponds to dipole or quadrupole modes. Also, if the system can be described in terms of a single particle per unit-cell, the sum in $\nu \to j$ can be disregarded and the expressions for the structure factors $S$ can be obtained by substituting $\vec{R}_{j,j'} \to \vec{R}$.

## 3.2 Plasmon-Photon Interactions

Let us now consider the collective interaction of the nanoparticle supercrystal with photons. We will first apply the usual Taylor's expansion of the vector potential and then apply the expansion in spherical harmonics.

### 3.2.1 Taylor's Series Expansion

*Dipole-Photon interaction*

The dipole-photon interaction term is

$$\mathcal{H}^{D}_{\text{plpt}} = \sum_{\vec{R},j,\lambda\sigma} \frac{1}{M_j}\Pi_{\vec{R},j,\sigma}\mathrm{Q}^D_j A_\lambda(\vec{R}_j)(\hat{e}_\sigma\cdot\hat{e}_\lambda) + \frac{1}{2M_j^2}\mathrm{Q}^D_j\mathrm{Q}^D_j A_\lambda(\vec{R}_j)A_\lambda(\vec{R}_j)(\hat{e}_\lambda\cdot\hat{e}_{\lambda'}), \tag{S.3.31}$$

where

$$A_\lambda(\vec{R}_j) = \sum_{\vec{q}}\sqrt{\frac{\hbar}{2\epsilon_m\epsilon_0 V\omega_{pt}(\vec{q})}}\left(c_{\vec{q},\lambda}e^{i\vec{q}\cdot\vec{R}_j} + c^\dagger_{\vec{q},\lambda}e^{-i\vec{q}\cdot\vec{R}_j}\right). \tag{S.3.32}$$

Substituting the plasmon momentum

$$\Pi_{\vec{R},j,\sigma} = -i\sqrt{\frac{\hbar M_j\omega^D_j}{2N}}\sum_{\vec{q}}\left(b_{\vec{q},j,\sigma}e^{i\vec{q}\cdot\vec{R}_j} - b^\dagger_{\vec{q},j,\sigma}e^{-i\vec{q}\cdot\vec{R}_j}\right), \tag{S.3.33}$$

into this equation, we find the linear first-order contribution to the dipole-photon interaction

$$\begin{aligned}
\mathcal{H}^{(D,1)}_{\text{plpt}} &= \sum_{\vec{R},j,\vec{q},\vec{q}',\lambda,\sigma} i\sqrt{\frac{\hbar^2 M_j\omega^D_j}{4\epsilon_m\epsilon_0 NV\omega_{pt}(\vec{q})M_j^2}}\mathrm{Q}^D_j(\hat{e}_\sigma\cdot\hat{e}_\lambda)\\
&\times\Big[b^\dagger_{\vec{q},j,\sigma}c_{\vec{q}',\lambda}e^{i(\vec{q}'-\vec{q})\cdot\vec{R}_j} - b_{\vec{q},j,\sigma}c_{\vec{q}',\lambda}e^{i(\vec{q}'+\vec{q})\cdot\vec{R}_j} +\\
&\quad + b^\dagger_{\vec{q},j,\sigma}c^\dagger_{\vec{q}',\lambda}e^{-i(\vec{q}'+\vec{q})\cdot\vec{R}_j} - b_{\vec{q},j,\sigma}c^\dagger_{\vec{q}',\lambda}e^{-i(\vec{q}'-\vec{q})\cdot\vec{R}_j}\Big]\\
&= \sum_{j,\vec{q},\vec{G},\lambda,\sigma} i\hbar\omega^D_j\sqrt{\frac{2\pi(\mathrm{Q}^D_j)^2}{8\pi\epsilon_m\epsilon_0 V_{UC}\omega_{pt}(\vec{q})M_j\omega^D_j}}(\hat{e}_\sigma\cdot\hat{e}_\lambda)\\
&\times\Big[b^\dagger_{\vec{q},j,\sigma}c_{\vec{q}+\vec{G},\lambda} - b_{\vec{q},j,\sigma}c_{-\vec{q}-\vec{G},\lambda} + b^\dagger_{\vec{q},j,\sigma}c^\dagger_{-\vec{q}-\vec{G},\lambda} - b_{\vec{q},j,\sigma}c^\dagger_{\vec{q}+\vec{G},\lambda}\Big]\\
&= \sum_{j,\vec{q},\vec{G},\lambda,\sigma} i\hbar\omega^D_j\xi^{\sigma,j}_{\lambda\vec{G}}(\vec{q})\Big[b^\dagger_{-\vec{q},j,\sigma}c_{-\vec{q}-\vec{G},\lambda} - b_{\vec{q},j,\sigma}c_{-\vec{q}-\vec{G},\lambda} +\\
&\quad + b^\dagger_{-\vec{q},j,\sigma}c^\dagger_{\vec{q}+\vec{G},\lambda} - b_{\vec{q},j,\sigma}c^\dagger_{\vec{q}+\vec{G},\lambda}\Big],
\end{aligned} \tag{S.3.34}$$

where we have used $\sum_{\vec{R}_j}\exp[i(\vec{q}\mp\vec{q}')\cdot\vec{R}']/N = \delta_{\vec{q}',\pm\vec{q}\pm\vec{G}}$, with $\vec{G}$ a reciprocal lattice vector. Here, we defined the light-matter coupling term

$$\xi^{\sigma,j}_{\lambda\vec{G}}(\vec{q}) = \sqrt{\frac{2\pi\Lambda_{D,j}}{\omega_{pt}(\vec{q}+\vec{G})}}P_{\sigma\lambda}(\vec{q}+\vec{G}), \tag{S.3.35}$$

where the polarization function $P_{\sigma\lambda}(\vec{q}+\vec{G})$ ensures that the photon polarization is perpendicular to its wavevector.

Following the work of Lamowski *et al.*[2], we define the two possible photon polarizations as

$$\begin{cases} \hat{e}_{\lambda_1} = \hat{e}_z \times \hat{e}_q \\ \hat{e}_{\lambda_2} = \hat{e}_q \times \hat{e}_{\lambda_1} \end{cases}, \tag{S.3.36}$$

for $\hat{e}_q \parallel \hat{e}_z$, we assume $\lambda_1 \parallel x$.

Finally, we can cast this term into the form

$$\mathcal{H}^{(D,1)}_{\text{plpt}} = \sum_{j,\vec{q},\lambda\sigma} i\hbar\omega_j^D \xi^{\sigma,j}_{\lambda\vec{G}}(\vec{q}) \left(b^\dagger_{-\vec{q},j,\sigma} - b_{\vec{q},j,\sigma}\right)\left(c^\dagger_{\vec{q}+\vec{G},\lambda} + c_{-\vec{q}-\vec{G},\lambda}\right). \tag{S.3.37}$$

For the second-order term it is useful to write $\vec{q} \to \vec{q} + \vec{G}$ and $\vec{q}' \to \vec{q}' + \vec{G}'$, leading to

$$\begin{aligned} \mathcal{H}^{(D,2)}_{\text{plpt}} &= \sum_{j,\vec{q},\sigma\lambda} \frac{\hbar}{4M_j\epsilon_m\epsilon_0 V_{\text{UC}}\sqrt{\omega_{pt}(\vec{q})\omega_{pt}(\vec{q}')}} \text{Q}_j^D \text{Q}_j^D \Big[c^\dagger_{-\vec{q},\lambda}c_{-\vec{q}',\lambda} + c_{\vec{q},\lambda}c_{-\vec{q}',\lambda} + \\ &\quad + c^\dagger_{-\vec{q},\lambda}c^\dagger_{\vec{q}',\lambda} + c_{\vec{q},\lambda}c^\dagger_{\vec{q}',\lambda}\Big] \\ &= \sum_{j,\vec{q},\sigma,\lambda,\lambda',\vec{G},\vec{G}'} \hbar\omega_j^D \xi^{\sigma,j*}_{\lambda',\vec{G}'}(\vec{q})\xi^{\sigma,j}_{\lambda\vec{G}}(\vec{q}) \left(c^\dagger_{-\vec{q}-\vec{G}',\lambda} + c_{\vec{q}+\vec{G}',\lambda}\right)\left(c_{-\vec{q}-\vec{G},\lambda} + c^\dagger_{\vec{q}+\vec{G},\lambda}\right), \end{aligned} \tag{S.3.38}$$

where we have used the following relation

$$[\hat{e}_{\lambda'}(\vec{q}+\vec{G}')\cdot\hat{e}_\lambda(\vec{q}+\vec{G})] = \sum_\sigma P_{\lambda\sigma}(\vec{q}+\vec{G})P_{\lambda'\sigma}(\vec{q}+\vec{G}'). \tag{S.3.39}$$

With this, we obtain the dipole-photon interaction terms

$$\mathcal{H}^{(D,1)}_{\text{plpt}} = i\hbar \sum_{j,\vec{q},\vec{G},\lambda,\sigma} \omega_j^D \xi^{\sigma,j}_{\lambda\vec{G}} \left(b^\dagger_{-\vec{q},j,\sigma} - b_{\vec{q},j,\sigma}\right)\left(c_{-\vec{q}-\vec{G},\lambda} + c^\dagger_{\vec{q}+\vec{G},\lambda}\right), \tag{S.3.40}$$

and

$$\mathcal{H}^{(D,2)}_{\text{plpt}} = \hbar \sum_{\vec{q},\lambda\vec{G},\vec{G}'} \Xi^{D,\lambda\lambda'}_{\vec{G},\vec{G}'}(\vec{q}) \left(c^\dagger_{-\vec{q}-\vec{G}',\lambda'} + c_{\vec{q}+\vec{G}',\lambda'}\right)\left(c_{-\vec{q}-\vec{G},\lambda} + c^\dagger_{\vec{q}+\vec{G},\lambda}\right), \tag{S.3.41}$$

where we have defined

$$\Xi^{D,\lambda\lambda'}_{\vec{G}\vec{G}'}(\vec{q}) = \sum_{j,\sigma} \omega_j^D \xi^{\sigma,j*}_{\lambda',\vec{G}'}(\vec{q})\xi^{\sigma,j}_{\lambda\vec{G}}(\vec{q}) = \Xi^{D,\lambda\lambda'*}_{\vec{G}\vec{G}'}(\vec{q}). \tag{S.3.42}$$

These equations imply that the plasmonic states with wavevector $\vec{q}$ are coupled with all photon states with wavevectors given by $\vec{q}+\vec{G}$. With this, the dynamical matrix, which needs to be diagonalized within the Boguliobov transformation, must account for the different possible values of $\vec{G}$.

*Quadrupole-Photon Interaction*

To calculate the interaction of light with the quadrupole modes we first evaluate the dyadic gradient $\nabla A(R)$. For this, we start with

$$\vec{A}(\vec{r}) = \sum_{\vec{q},\lambda} \sqrt{\frac{\hbar}{2\epsilon_m\epsilon_0 V\omega_{pt}(\vec{q})}} \left(c_{\vec{q},\lambda} e^{i\vec{q}\cdot\vec{r}} + c^{\dagger}_{\vec{q},\lambda} e^{-i\vec{q}\cdot\vec{r}}\right), \tag{S.3.43}$$

so that

$$[\nabla A(\vec{R}_j)]_{\alpha\beta} = \frac{\partial}{\partial x_\beta} A_\alpha = i \sum_{\vec{q}} \sqrt{\frac{\hbar}{2\epsilon_m\epsilon_0 V\omega_{pt}(\vec{q})}} q_\beta \left(c_{\vec{q},\alpha} e^{i\vec{q}\cdot\vec{R}_j} - c_{\vec{q},\alpha} e^{-i\vec{q}\cdot\vec{R}_j}\right), \tag{S.3.44}$$

where $R_j$ is the position of the $j$-th particle in the unit cell defined by the vector $\vec{R}$. This leads to

$$[\nabla A(\vec{R}_j)] = \sum_{\vec{q}\lambda} iq \sqrt{\frac{\hbar}{2\epsilon_m\epsilon_0 V\omega_{pt}(q)}} \left(c_{\vec{q},\lambda} e^{i\vec{q}\cdot\vec{r}} + c^{\dagger}_{-\vec{q},\lambda} e^{-i\vec{q}\cdot\vec{r}}\right) \hat{e}_q \hat{e}_\lambda. \tag{S.3.45}$$

We now expand the quadrupole momentum operator $\Pi_{\vec{R},j,\sigma}$ in Bloch functions

$$\begin{aligned}\mathcal{H}^{(Q,1)}_{plpt} = \sum_{q',q,j,\lambda\gamma} &-\frac{\mathrm{q}'}{2M_j c} \sqrt{\frac{\hbar}{2\epsilon_m\epsilon_0 V\omega_{pt}(\vec{q})}} \sqrt{\frac{\hbar M_j \omega^D_j}{2}} \mathrm{Q}^Q_j \bar{\rho}_j \left(b_{\vec{q},j,\gamma} e^{i\vec{q}\vec{R}} - b^{\dagger}_{-\vec{q},j,\gamma} e^{-i\vec{q}\vec{R}}\right) \\ &\times \left(c_{\vec{q}',\lambda} e^{i\vec{q}'\cdot\vec{r}} + c^{\dagger}_{-\vec{q}',\lambda} e^{-i\vec{q}'\cdot\vec{r}}\right) [\chi_\gamma : \hat{e}_q \hat{e}_\lambda].\end{aligned} \tag{S.3.46}$$

We can then follow the steps from the light-dipole interaction to define

$$\xi^{\gamma,j}_{\lambda\vec{G}}(\vec{q}) = i \sqrt{\frac{2\pi\Lambda_{Q,j}}{\omega_{pt}(\vec{q}+\vec{G})}} |\vec{q}+\vec{G}| \bar{R} \, [\chi_\gamma : \hat{e}_q \hat{e}_\lambda]. \tag{S.3.47}$$

The interaction now has the same overall shape as that of the first-order term in the light-dipole interaction

$$\mathcal{H}^{Q,(1)}_{plpt} = \sum_{q,G,j,\gamma,\lambda} i\hbar\omega^D_j \xi^Q_{j,\vec{G}}(\vec{q}) \left(b_{\vec{q},j,\sigma} - b^{\dagger}_{-\vec{q},j,\sigma}\right) \left(c_{\vec{q}+\vec{G},\lambda} + c^{\dagger}_{-\vec{q}-\vec{G},\lambda}\right), \tag{S.3.48}$$

with a different definition of the coupling matrix $\xi$.

We note that the dyadic $\hat{e}_q \hat{e}_\lambda$ is not symmetric. It is then interesting to write it as a sum of a symmetric and an anti-symmetric part

$$\hat{e}_q \hat{e}_\lambda = \frac{\hat{e}_q \hat{e}_\lambda + \hat{e}_\lambda \hat{e}_q}{2} + \frac{\hat{e}_q \hat{e}_\lambda - \hat{e}_\lambda \hat{e}_q}{2}. \tag{S.3.49}$$

Since $\chi_\gamma$ is always symmetric, its dot product with the anti-symmetric part is always zero. We define

$$P^Q_{\gamma\lambda}(\vec{q}) = \frac{1}{2}[\chi_\gamma : \hat{e}_q \hat{e}_\lambda + \hat{e}_\lambda \hat{e}_q], \tag{S.3.50}$$

to get

$$\xi^{\gamma,j}_{\lambda\vec{G}}(\vec{q}) = i\sqrt{\frac{2\pi\Lambda_{Q,j}}{\omega_{pt}(\vec{q}+\vec{G})}}|\vec{q}+\vec{G}|\bar{R}P^{Q}_{\gamma\lambda}(\vec{q}). \tag{S.3.51}$$

For the second-order contribution, we note that the dot product between the two dyadic gradients is

$$\begin{aligned}\nabla A^{\dagger}(\vec{R}_j)\cdot\nabla A(\vec{R}_j) = \sum_{\vec{q}\lambda q'\lambda'} qq'\frac{\hbar}{2\epsilon_m\epsilon_0 V\sqrt{\omega_{pt}(q)\omega_{pt}(q')}}\left(c_{\vec{q},\lambda}e^{i\vec{q}\cdot\vec{r}} + c^{\dagger}_{-\vec{q},\lambda}e^{-i\vec{q}\cdot\vec{r}}\right) \\ \times\left(c_{\vec{q}',\lambda'}e^{i\vec{q}\cdot\vec{r}} + c^{\dagger}_{-\vec{q}',\lambda'}e^{-i\vec{q}'\cdot\vec{r}}\right)[\hat{e}_q\hat{e}_{\lambda}\cdot\hat{e}_{\lambda'}\hat{e}_{q'}].\end{aligned} \tag{S.3.52}$$

We exchange each of these dyadics by their symmetric parts, as done for the first-order term, and use the completeness of the $\chi$ matrices for symmetric tensors to write

$$[\hat{e}_q\hat{e}_{\lambda}\cdot\hat{e}_{\lambda'}\hat{e}_{q'}] = \sum_{\gamma\gamma'} P^{Q}_{\gamma\lambda}(\vec{q})[\chi_{\gamma}\cdot\chi_{\gamma'}]P^{Q}_{\gamma'\lambda'}(\vec{q}'). \tag{S.3.53}$$

This leads to

$$[1:(\hat{e}_q\hat{e}_{\lambda}\cdot\hat{e}_{\lambda'}\hat{e}_{q'})] = \sum_{\gamma\gamma'} P^{Q}_{\gamma\lambda}(\vec{q})P^{Q}_{\gamma'\lambda'}(\vec{q}')\delta_{\gamma,\gamma'} = \sum_{\gamma} P^{Q}_{\gamma\lambda}(\vec{q})P^{Q}_{\gamma\lambda'}(\vec{q}'). \tag{S.3.54}$$

Finally, we can follow the same procedures as before to arrive at

$$\mathcal{H}^{(Q,2)}_{\text{plpt}} = \hbar\sum_{\vec{q},\lambda\lambda'\vec{G},\vec{G}'\gamma} \omega^{Q}_{j}\xi^{\gamma\lambda'*}_{j,\vec{G}'}(\vec{q})\xi^{\gamma,j}_{\lambda\vec{G}}(\vec{q})\left(c^{\dagger}_{-\vec{q}-\vec{G}',\lambda'} + c_{\vec{q}+\vec{G}',\lambda'}\right)\left(c_{-\vec{q}-\vec{G},\lambda} + c^{\dagger}_{\vec{q}+\vec{G},\lambda}\right). \tag{S.3.55}$$

The final expressions for the quadrupole-photon interaction can now be written as

$$\mathcal{H}^{Q,(1)}_{\text{plpt}} = i\hbar\sum_{j,\vec{q},\vec{G},\lambda,\gamma} \omega^{Q}_{j}\xi^{\gamma,j}_{\lambda\vec{G}}\left(b^{\dagger}_{-\vec{q},j,\sigma} - b_{\vec{q},j,\sigma}\right)\left(c_{-\vec{q}-\vec{G},\lambda} + c^{\dagger}_{\vec{q}+\vec{G},\lambda}\right), \tag{S.3.56}$$

and

$$\mathcal{H}^{(Q,2)}_{\text{plpt}} = \hbar\sum_{\vec{q},\lambda\vec{G},\vec{G}'} \Xi^{Q,\lambda\lambda'}_{\vec{G},\vec{G}'}(\vec{q})\left(c^{\dagger}_{-\vec{q}-\vec{G}',\lambda} + c_{\vec{q}+\vec{G}',\lambda}\right)\left(c_{-\vec{q}-\vec{G},\lambda} + c^{\dagger}_{\vec{q}+\vec{G},\lambda}\right), \tag{S.3.57}$$

where we have defined

$$\Xi^{Q,\lambda\lambda'}_{\vec{G}\vec{G}'}(\vec{q}) = \sum_{j\gamma}\omega_j\xi^{\gamma,j*}_{\lambda',\vec{G}'}(\vec{q})\xi^{\gamma,j}_{\lambda\vec{G}}(\vec{q}) = \Xi^{Q,\lambda\lambda'*}_{\vec{G}\vec{G}'}(\vec{q}). \tag{S.3.58}$$

It is interesting to note that the ratio between the contributions from other BZs compared to the 1st BZ scale as $\sqrt{|\vec{q}+\vec{G}|/|\sqrt{q}|}$. Contrary to the dipole-light interaction, which decreases by $\sim 1/\sqrt{|\vec{G}|}$ as we move away from the 1st BZ, the dipole quadrupole interaction actually increases by $\sqrt{\vec{G}}$, and does not converge. This indicates that for particles with sizes comparable to the lattice parameter, keeping only first-order terms in $\vec{q}$ on the Taylor expansion of the vector potential $\vec{A}$ (quadrupole approximations) will lead to unphysical results, demonstrating the need for the spherical harmonic expansion.

### 3.2.2 Spherical Harmonic Expansion of the Vector Potential

It is straightforward to show that the light-matter coupling parameters simply get re-scaled by the form factors $\mathrm{f}_D(\vec{q})$ and $\mathrm{f}_Q(q)$, and thus can be written as

$$\xi^{\sigma,j}_{\lambda\vec{G}}(\vec{q}) = \mathrm{f}_D(|\vec{q}+\vec{G}|\rho)\sqrt{\frac{2\pi\Lambda_{D,j}}{\omega_{pt}(\vec{q}+\vec{G})}}e^{-i\vec{G}\cdot\vec{r}_j}P_{\sigma\lambda}(\vec{q}+\vec{G}), \tag{S.3.59}$$

and

$$\xi^{\gamma,j}_{\lambda\vec{G}}(\vec{q}) = i\mathrm{f}_Q(|\vec{q}+\vec{G}|\rho)\sqrt{\frac{2\pi\Lambda_{Q,j}}{\omega_{pt}(\vec{q}+\vec{G})}}e^{-i\vec{G}\cdot\vec{r}_j}|\vec{q}+\vec{G}|\bar{R}P^Q_{\gamma\lambda}(\vec{q}+\vec{G}). \tag{S.3.60}$$

Here, we have defined

$$\xi^{\bar{\nu}}_0(\vec{q}) = \sqrt{\frac{2\pi\Lambda_{\bar{\nu}}}{\omega_{pt}(\vec{q})}}, \tag{S.3.61}$$

where $\bar{\nu} = D,\ Q$ for dipole/quadrupole plasmons. We can also write more concise equations for the coupling constants

$$\xi^{D,\nu}_{\lambda,\vec{G}}(\vec{q}) = \mathrm{f}_D(|\vec{q}+\vec{G}|)\xi^D_0(\vec{q})P^D_{\lambda,\nu}(\vec{q}+\vec{G}), \tag{S.3.62}$$

and

$$\xi^{Q,\nu}_{\lambda,\vec{G}}(\vec{q}) = i\mathrm{f}_Q(|\vec{q}+\vec{G}|)|\vec{q}+\vec{G}|\bar{R}\xi^Q_0(\vec{q})P^Q_{\lambda,\nu}(\vec{q}+\vec{G}), \tag{S.3.63}$$

where the index $j$ was suppressed. For the second-order processes, we will have the exact same equations but with the modified expressions for $\xi(\vec{q})$.

### 3.2.3 General Plasmon-Photon Interaction

We combine all results obtained into a general expression for both the first-order and second-order parts of the Hamiltonian as

$$\mathcal{H}^{(1)}_{\mathrm{plpt}} = i\hbar\sum_{\vec{q},\vec{G},\lambda,\nu}\omega_\nu\xi^{\nu,j}_{\lambda\vec{G}}\left(b^\dagger_{-\vec{q},j,\nu} - b_{\vec{q},j,\nu}\right)\left(c_{-\vec{q}-\vec{G},\lambda} + c^\dagger_{\vec{q}+\vec{G},\lambda}\right), \tag{S.3.64}$$

and

$$\mathcal{H}^{(ii)}_{\mathrm{plpt}} = \hbar\sum_{\vec{q},\lambda\vec{G},\vec{G}'}\Xi^{\lambda\lambda'}_{\vec{G}\vec{G}'}(\vec{q})\left(c^\dagger_{-\vec{q}-\vec{G}',\lambda'} + c_{\vec{q}+\vec{G}',\lambda'}\right)\left(c_{-\vec{q}-\vec{G},\lambda} + c^\dagger_{\vec{q}+\vec{G},\lambda}\right), \tag{S.3.65}$$

where

$$\xi^{D,j}_{\lambda\vec{G}}(\vec{q}) = \mathrm{f}_{D,j}(|\vec{q}+\vec{G}|)\xi^D_0(\vec{q})P^D_\lambda(\vec{q}+\vec{G}), \tag{S.3.66}$$

and

$$\xi^Q_{\lambda,j,\vec{G}}(\vec{q}) = i\mathrm{f}_{Q,j}(|\vec{q}+\vec{G}|)|\vec{q}+\vec{G}|\bar{R}\xi^Q_{0,j}(\vec{q})P^Q_\lambda(\vec{q}+\vec{G}). \tag{S.3.67}$$

Here,

$$\xi^{\nu}_{0,j}(\vec{q}) = \sqrt{\frac{2\pi\Lambda_{j,\bar{\nu}}}{\omega_{pt}(\vec{q})}}, \tag{S.3.68}$$

and

$$\Xi^{\lambda\lambda'}_{\vec{G}\vec{G}'}(\vec{q}) = \sum_{\nu,j} \omega_{j,\bar{\nu}} \xi^{\nu,j*}_{\lambda'\vec{G}'}(\vec{q}) \xi^{\nu,j}_{\lambda,\vec{G}}(\vec{q}). \tag{S.3.69}$$

The index $\nu$ runs through the possible plasmon states of the $j$-th particle in the unit cell, $\vec{G}$ runs through the considered Brillouin zones, and $\lambda$ runs through the polarizations perpendicular to the wave vector $\vec{q} + \vec{G}$. If one considers only one atom in the unit cell, the $j$ label becomes irrelevant, leading to the simpler expressions used in the main manuscript.

# 4 Bogoliubov Transformation

In this section we describe the process for organizing the terms in the total Hamiltonian to match the formalism developed by Xiao *et al.* [3] for quadratic Hamiltonians.

The Hamiltonian needs to be written in the form

$$\mathcal{H} = E_0 + \hbar \sum_{i,j=1}^{n+1} \left( \alpha_{ij} d_i^\dagger d_j + \frac{1}{2}\gamma_{ij} d_i^\dagger d_j^\dagger + \frac{1}{2}\gamma_{ij}^* d_i d_j \right). \tag{S.4.1}$$

We must find the appropriate matrices $\alpha$ and $\gamma$ written as

$$\alpha_{\tilde{\mathbf{q}}} = \begin{pmatrix} \alpha_{plpl}(\vec{q}) & \alpha_{plpt}(\vec{q}) \\ \alpha^\dagger_{plpt}(\vec{q}) & \alpha_{ptpt}(\vec{q}) \end{pmatrix}, \gamma_{\tilde{\mathbf{q}}} = \begin{pmatrix} \gamma_{plpl}(\vec{q}) & \gamma_{plpt}(\vec{q}) \\ \gamma^t_{plpt}(\vec{q}) & \gamma_{ptpt}(\vec{q}) \end{pmatrix}. \tag{S.4.2}$$

The contribution of the bare plasmon and photon terms in the Hamiltonian are trivial. We will start with the plasmon-plasmon interaction. The general plasmon-plasmon Hamiltonian term is

$$\begin{aligned} \mathcal{H}_{\text{plpl}} &= \sum_{\nu,\nu',\vec{q},} \hbar\mathcal{S}_{\nu\nu'} \left[ b^\dagger_{\vec{q},\nu} b^\dagger_{-\vec{q},\nu'} + b^\dagger_{\vec{q},\nu} b_{\vec{q},\nu'} + b_{\vec{q},\nu} b^\dagger_{\vec{q},\nu'} + b_{\vec{q},\nu} b_{-\vec{q},\nu'} \right]. \\ &= \sum_{\nu,\nu',\vec{q}} \hbar\mathcal{S}_{\nu,\nu'}(\vec{q}) \left\{ \left[ 2b^\dagger_{\vec{q},\nu} b_{\vec{q},\nu'} + b^\dagger_{\vec{q},\nu} b^\dagger_{-\vec{q},\nu'} + b_{-\vec{q},\nu} b_{\vec{q},\nu'} \right] - \delta_{j,j'}\delta_{\sigma,\sigma'} \right\} \\ &= \sum_{\nu,\nu',\vec{q}\in Z} \hbar\mathcal{S}_{\nu,\nu'}(\vec{q}) \left\{ \left[ 2b^\dagger_{\vec{q},\nu} b_{\vec{q},\nu'} + b^\dagger_{\vec{q},\nu} b^\dagger_{-\vec{q},\nu'} + b_{-\vec{q},\nu} b_{\vec{q},\nu'} \right] + \right. \\ &\quad \left. \hbar\mathcal{S}_{\nu,\nu'}(-\vec{q}) + \left[ 2b_{-\vec{q},\nu} b^\dagger_{-\vec{q},\nu'} + b^\dagger_{-\vec{q},\nu} b^\dagger_{\vec{q},\nu'} + b_{\vec{q},\nu} b_{-\vec{q},\nu'} \right] \right\}, \end{aligned} \tag{S.4.3}$$

where we have defined the sub-space $Z$ that is spanned by the half space of positive $\vec{q}$, such that if $\vec{q} \in Z$ then $-\vec{q} \notin Z$. This subset excludes the $\Gamma$ ($q = 0$) point. What happens at this point will be discussed later. For now, it can be simply avoided in the calculations or considered as the limiting case $\vec{q} \to 0$. We defined the plasmon-plasmon coupling tensor

$$\mathcal{S}_{\nu,\nu'}(\vec{q}) = \sqrt{\Lambda_{\bar{\nu}}\Lambda_{\bar{\nu}'}} S^{\bar{\nu}\bar{\nu}'}_{\nu,\nu'}(\vec{q}). \tag{S.4.4}$$

By inspection, we can see that $\mathcal{H}_{\rm plpl}$ can be rewritten into the form of Eq. (S.4.1) by defining

$$\begin{aligned}\alpha_{plpl}(\vec{q}) =&\bar{\omega}_{pl} + 2\bar{\mathcal{S}}_{\vec{q}}\\ \gamma_{plpl}(\vec{q}) =&\bar{\mathcal{S}}_{\vec{q}} + \bar{\mathcal{S}}^*_{\vec{q}},\end{aligned} \tag{S.4.5}$$

where we used $\mathcal{S}_{-\vec{q}} = \mathcal{S}^*_{\vec{q}}$.

The plasmon-photon interaction is

$$\begin{aligned}\mathcal{H}^{(1)}_{\rm plpt} =&i\hbar \sum_{j,\nu,\lambda,\vec{G},\vec{q}\in Z} \omega^{\nu}_{j}\xi^{\nu\lambda}_{j,\vec{G}}(\vec{q})\left[b^{\dagger}_{-\vec{q},j,\nu}c_{-\vec{q}-\vec{G},\lambda} - c^{\dagger}_{\vec{q}+\vec{G},\lambda}b_{\vec{q},j,\nu} + c^{\dagger}_{\vec{q}+\vec{G},\lambda}b^{\dagger}_{-\vec{q},j,\nu} - b_{\vec{q},j,\nu}c_{-\vec{q}-\vec{G},\lambda}\right]\\ &+ \omega^{\nu}_{j}\xi^{\nu\lambda}_{j,\vec{G}}(-\vec{q})\left[b^{\dagger}_{\vec{q},j,\nu}c_{\vec{q}-\vec{G},\lambda} - c^{\dagger}_{-\vec{q}+\vec{G},\lambda}b_{-\vec{q},j,\nu} + c^{\dagger}_{-\vec{q}+\vec{G},\lambda}b^{\dagger}_{\vec{q},j,\nu} - b_{-\vec{q},j,\nu}c_{\vec{q}-\vec{G},\lambda}\right],\end{aligned} \tag{S.4.6}$$

leading to

$$\alpha_{plpt}(\vec{q}) = i\hbar\omega_{\nu}\xi^{\nu\lambda}_{\vec{G}}. \tag{S.4.7}$$

The second-order term has the generalized form

$$\begin{aligned}\mathcal{H}^{(ii)}_{\rm plpt} =&\hbar \sum_{\vec{q},\vec{G},\vec{G}',\lambda,\lambda'} \Xi^{\lambda\lambda'}_{\vec{G}\vec{G}'}(\vec{q})\left[c^{\dagger}_{-\vec{q}-\vec{G}',\lambda'}c_{-\vec{q}-\vec{G},\lambda} + c^{\dagger}_{-\vec{q}-\vec{G}',\lambda'}c^{\dagger}_{\vec{q}+\vec{G},\lambda} + c_{\vec{q}+\vec{G}',\lambda'}c_{-\vec{q}-\vec{G},\lambda} + c_{\vec{q}+\vec{G}',\lambda'}c^{\dagger}_{\vec{q}+\vec{G},\lambda}\right]\\ =&\hbar \sum_{\vec{G},\vec{G}',\lambda,\lambda',\vec{q}\in Z} \Xi^{\lambda\lambda'}_{\vec{G}\vec{G}'}(\vec{q})\left[c^{\dagger}_{-\vec{q}-\vec{G}',\lambda'}c_{-\vec{q}-\vec{G},\lambda} + c^{\dagger}_{-\vec{q}-\vec{G}',\lambda'}c^{\dagger}_{\vec{q}+\vec{G},\lambda} + c_{\vec{q}+\vec{G}',\lambda'}c_{-\vec{q}-\vec{G},\lambda} + c_{\vec{q}+\vec{G}',\lambda'}c^{\dagger}_{\vec{q}+\vec{G},\lambda}\right]\\ &+ \sum_{\vec{G},\vec{G}',\lambda,\lambda',\vec{q}\in Z} \Xi^{\lambda\lambda'}_{\vec{G}\vec{G}'}(\vec{q})\left[c^{\dagger}_{\vec{q}+\vec{G}',\lambda'}c_{\vec{q}+\vec{G},\lambda} + c^{\dagger}_{\vec{q}+\vec{G}',\lambda'}c^{\dagger}_{-\vec{q}-\vec{G},\lambda} + c_{-\vec{q}-\vec{G}',\lambda'}c_{\vec{q}+\vec{G},\lambda} + c_{-\vec{q}-\vec{G}',\lambda'}c^{\dagger}_{-\vec{q}-\vec{G},\lambda}\right]\\ =&\ \hbar \sum_{\vec{G},\vec{G}',\lambda,\lambda,\vec{q}\in Z} \Xi^{\lambda\lambda'}_{\vec{G}\vec{G}}(\vec{q})\left[2c^{\dagger}_{\vec{q}+\vec{G},\lambda}c_{\vec{q}+\vec{G},\lambda} + c^{\dagger}_{-\vec{q}-\vec{G},\lambda}c^{\dagger}_{\vec{q}+\vec{G},\lambda} + c_{\vec{q}+\vec{G},\lambda}c_{-\vec{q}-\vec{G},\lambda}\right]\\ &+ \Xi^{\lambda\lambda'}_{\vec{G}\vec{G}}(\vec{q})\left[2c_{-\vec{q}-\vec{G},\lambda}c^{\dagger}_{-\vec{q}-\vec{G},\lambda} + c^{\dagger}_{\vec{q}+\vec{G},\lambda}c^{\dagger}_{-\vec{q}-\vec{G},\lambda} + c_{-\vec{q}-\vec{G},\lambda}c_{\vec{q}+\vec{G},\lambda}\right].\end{aligned} \tag{S.4.8}$$

It is convenient to define the $2N_{\vec{G}} \times 2N_{\vec{G}}$ matrix $\bar{\Xi}_{\vec{q}} = \bar{\xi}^{\dagger}\bar{\omega}_{pl}\bar{\xi}$. With this, we write the Xiao matrices for the photon states as

$$\begin{aligned}\alpha_{ptpt}(\vec{q}) =&\bar{\omega}_{pt} + 2\bar{\Xi}_{\vec{q}}\\ \gamma_{ptpt}(\vec{q}) =&\bar{2}\Xi_{\vec{q}},\end{aligned} \tag{S.4.9}$$

where we used $\Xi_{\vec{q}} = \Xi_{-\vec{q}}$.

We find that the matrices $\alpha_{\vec{q}}$ and $\gamma_{\vec{q}}$ can be written in compact form

$$\alpha_{\mathbf{\tilde{q}}} = \begin{pmatrix}\bar{\omega}_{pl} + 2\bar{\mathcal{S}}_{\vec{q}} & \bar{\omega}_{pl}\bar{\xi}_{\vec{q}}\\ \bar{\omega}_{pl}\bar{\xi}^{\dagger}_{\vec{q}} & \bar{\omega}^{pt}_{\vec{q}} + 2\bar{\Xi}_{\vec{q}}\end{pmatrix}, \gamma_{\mathbf{\tilde{q}}} = \begin{pmatrix}2\bar{\mathcal{S}}_{\vec{q}} & \bar{\omega}_{pl}\bar{\xi}_{\vec{q}}(\vec{q})\\ -\bar{\omega}_{pl}\bar{\xi}^{\dagger}_{\vec{q}} & 2\bar{\Xi}_{\vec{q}}\end{pmatrix}, \tag{S.4.10}$$

with $\bar{\omega}_{pl} = \text{diag}[\omega_{\nu}]$ and $\bar{\omega}_{pt} = \text{diag}[\omega_{pt}(\vec{q} + \vec{G})]$ . This corresponds to defining the operator vector

$$\Phi_{\vec{q}} = \begin{pmatrix}\bar{b}_{\vec{q}}\\ \bar{c}_{\vec{q}}\\ \bar{b}^{\dagger}_{-\vec{q}}\\ \bar{c}^{\dagger}_{-\vec{q}}\end{pmatrix}, \tag{S.4.11}$$

where $\bar{b}_{\vec{q}}$, $\bar{b}^{\dagger}_{-\vec{q}}$, are column vectors with each entry being an operator corresponding to different values of $\nu$ and $\bar{c}_{\vec{q}}$, $\bar{c}^{\dagger}_{-\vec{q}}$ are column vectors with operators for each polarization $\lambda$ and each considered reciprocal lattice vector $\vec{G}$. With this, the Hamiltonian takes the form

$$\mathcal{H} = E_0 + \sum_{\vec{q}\in Z} \Phi^{\dagger}_{\vec{q}} \mathcal{H}_{\vec{q}} \Phi_{\vec{q}}, \tag{S.4.12}$$

with

$$\mathcal{H}_{\vec{q}} = \hbar \begin{pmatrix} \alpha_{\vec{q}} & \gamma_{\vec{q}} \\ \gamma^{\dagger}_{\vec{q}} & \alpha^{\star}_{\vec{q}} \end{pmatrix}. \tag{S.4.13}$$

Following Xiao *et al.*[3] we define the dynamic matrix $D$ as

$$D_{\vec{q}} = \hbar \begin{pmatrix} \alpha_{\vec{q}} & \gamma_{\vec{q}} \\ -\gamma^{\dagger}_{\vec{q}} & -\alpha^{\star}_{\vec{q}} \end{pmatrix}, \tag{S.4.14}$$

such that

$$i\hbar \frac{d}{dt} \Phi_{\vec{q}} = D_{\vec{q}} \Phi_{\vec{q}}. \tag{S.4.15}$$

With this, we can probe the dynamics of the systems by finding the Bogoliubov transformation $T_{\vec{q}}$ which takes the vector $\Phi_{\vec{q}}$ into $\Psi_{\vec{q}} = T_{\vec{q}} \Phi_{\vec{q}}$ such that

$$i\hbar \frac{d}{dt} \Psi_{\vec{q}} = \hbar\omega_{\vec{q}} \Psi_{\vec{q}}. \tag{S.4.16}$$

# 5 Quasistatic Properties

In the quasistatic approximation the frequencies for the dipole and quadrupole modes are

$$\omega_D = \frac{\omega_p}{\sqrt{\epsilon_d + 2\epsilon_m}}, \tag{S.5.1}$$

and

$$\omega_Q = \frac{\omega_p}{\sqrt{\epsilon_d + (3/2)\epsilon_m}}, \tag{S.5.2}$$

Based on the work by Doerr *et al.* [4] we find that a multipole inside a polarizable sphere with permittivity $\epsilon(\omega)$ embedded in a medium with constant permittivity $\epsilon_m$ is perceived, outside of the sphere, as having an effective multipole given by

$$\mathrm{Q_{lm}} = \frac{(2\mathrm{l}+1)\epsilon_{\mathrm{m}}}{\mathrm{l}\epsilon(\omega) + (\mathrm{l}+1)\epsilon_{\mathrm{m}}} \mathrm{Q}^0_{\mathrm{l,m}}. \tag{S.5.3}$$

The effective charge for dipole and quadrupole modes can be written as

$$\mathrm{Q}_D = \mathrm{Q} \frac{3\epsilon_m}{\epsilon_{d,j} + 2\epsilon_m}, \tag{S.5.4}$$

and

$$\mathrm{Q}_Q = \mathrm{Q}\frac{5}{2}\frac{\epsilon_m}{\epsilon_{d,j} + (3/2)\epsilon_m}. \tag{S.5.5}$$

With this we find the coupling constants for dipole and quadrupole modes

$$\Lambda_D = \frac{9\epsilon_m \omega_D}{8\pi(\epsilon_d + 2\epsilon_m)} F, \tag{S.5.6}$$

and

$$\Lambda_Q = \left(\frac{3}{4\pi}\right)^{5/3} \frac{5\epsilon_m \omega_Q}{12(\epsilon_d + (3/2)\epsilon_m)} F^{5/3}, \tag{S.5.7}$$

, where we defined the fill factor $F = 4\pi\rho^3/3V_{uc}$ as the ratio between the volume of the particle and the volume of the unit cell.

# 6 Umklapp Effects

Figure S1 shows the dependence of the plasmon-polariton energies as a function of the number of Brillouin zones ($nBZ$) considered for a given $q$. The energies are seen to converge for $nBZ > 4$. For all modes, the energies decrease with increasing $nBZ$. The energy changes are on the order of 50 - 100 meV. For the IPP and LPP bands this change can correspond to up to 10%, indicating that Umklapp effects are necessary for an accurate description of the plasmon-polaritons in the nanoparticle crystals.

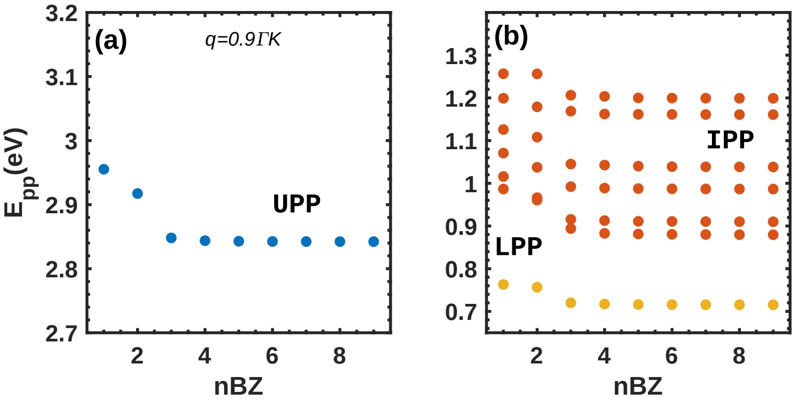


Figure S1: $nBZ$ dependence of the plasmon-polariton energies on the number of considered Brillouin zones ($nBZ$).

# References

[1] Aage Niels Bohr and Ben R Mottelson. Collective and individual-particle aspects of nuclear structure, 1953.

[2] Simon Lamowski, Charlie Ray Mann, Felicitas Hellbach, Eros Mariani, Guillaume Weick, and Fabian Pauly. Plasmon polaritons in cubic lattices of spherical metallic nanoparticles. *Physical Review B*, 97(12):1–11, 2018.

[3] Ming-wen Xiao. Theory of transformation for the diagonalization of quadratic Hamiltonians. *http://arxiv.org/abs/0908.0787*, 2009.

[4] T. P. Doerr, O. I. Obolensky, and Yi Kuo Yu. Extending electrostatics of dielectric spheres to arbitrary charge distributions with applications to biosystems. *Physical Review E*, 96(6), 2017.
